# Supplementary material for: Mixed Models with Multiple Instance Learning
Source: arXiv:2311.02455 ancillary file (2024-03-08)
Supplement: Supplementary file 1 [file appendix.pdf]

---

## Appendix for: “Attention-based Multi-instance Mixed Models”

---

### Contents

|      |                                     |   |
|------|-------------------------------------|---|
| A1   | GMIL training details               | 1 |
| A2   | Baseline models                     | 2 |
| A2.1 | MIL baselines                       | 2 |
| A2.2 | Traditional ML models               | 2 |
| A3   | Experimental setup                  | 2 |
| A3.1 | Simulations and Genomics dataset    | 2 |
| A3.2 | Microscopy dataset                  | 3 |
| A3.3 | Histopathology dataset              | 4 |
| A4   | Data processing                     | 4 |
| A4.1 | Variant filtering procedure         | 4 |
| A4.2 | Single-cell Embeddings              | 4 |
| A4.3 | Microscopy image feature extraction | 5 |
| A5   | Additional Results                  | 6 |
| A5.1 | Simulations                         | 6 |
| A5.2 | Single-cell Genomics dataset        | 7 |
| A5.3 | Microscopy dataset                  | 9 |

### A1 GMIL training details

To enhance numerical stability during training, we reparameterize the embedding-based prediction of our model. Specifically, introducing a bag-level index  $i$  to Eq (3-4) in the main text, we denote the embedding-based bag prediction of bag  $i$ , composed of  $I_i$  instances, as:

$$(\mathbf{u})_i = \mathbf{z}_\gamma(\mathbf{X}_i)^T \boldsymbol{\beta} \quad (\text{A.1})$$

where  $\mathbf{X}_i \in \mathbb{R}^{I_i \times Q}$  collectively denotes the instance embeddings in bag  $i$ . During training, we reparameterize the embedding-based prediction  $\mathbf{u}$  to have sample mean 0 and sample variance  $b^2 = \frac{1}{Q} \sum_{j=1}^Q \beta_j^2$ . Importantly, this reparameterization does not alter the model structure but improves its trainability and interpretability<sup>1</sup>. Specifically, we implement the reparameterization by first introducing

$$(\tilde{\mathbf{u}})_i = \mathbf{z}_\gamma(\mathbf{X}_i)^T \underbrace{\boldsymbol{\beta} / b}_{\boldsymbol{\eta}}, \quad (\text{A.2})$$

where  $\boldsymbol{\eta}$  has unit mean square. We then rescale  $\tilde{\mathbf{u}}$  to:

$$\mathbf{u} = b \times \frac{\tilde{\mathbf{u}} - \text{mean}(\tilde{\mathbf{u}})}{\text{std}(\tilde{\mathbf{u}})}. \quad (\text{A.3})$$

This standardization operation can be implemented within the Pytorch framework using a `batchnorm` layer. By doing so, we introduce stochasticity and stability during training, while keeping track of training set statistics for inference.

---

<sup>1</sup>After this reparameterization,  $\sigma_{\boldsymbol{\beta}}^2$  can be directly interpreted as the variance explained by pooled bag embeddings.

## A2 Baseline models

### A2.1 MIL baselines

- **ABMIL.** Ilse et al. (2018) use neural networks and attention to learn instance-specific weights and perform bag-level aggregation to optimize a downstream prediction task. The authors additionally propose a gated version of the model where they combine *tanh* and *sigmoid* activation functions to the attention weights to better learn non-linearities.
- **Additive MIL.** Javed et al. (2022) overcome the lack of weight interpretability by pooling instance-level predictions rather than pooling instance features. In greater detail, attention weights are first estimated similarly to ABMIL and used to weigh single instances in a bag. Successively, a predictor is applied directly to the weighted instances to derive instance-specific logits, which are summed to yield a bag-level prediction.
- **DSMIL.** Li et al. (2021) first model an instance classifier which provides class-specific activation scores for each element in a bag. Max-pooling on the classification scores defines a critical instance per class. To obtain bag-level embeddings, attention weights are learned based on the distance of single elements from the critical instance per class and used to aggregate features.
- **Bayes-MIL.** Cui et al. (2023) derive uncertainty over the attention weights of a standard MIL model by learning patch-specific posterior distributions with variational inference. In their application to histopathology screens, the authors introduce a slide regularizer to concentrate attention on either the positive or negative side of patches for precise localization with high confidence. Additionally, the authors encode spatial information between patches in Multiple Instance Learning (MIL) for Whole Slide Image (WSI) recognition and localization, proposing the use of Conditional Random Fields (CRF). Because spatial information is not available for the simulation, genetics and microscopy datasets, we use the Bayes-MIL version without slide regularizer and CRF.

### A2.2 Traditional ML models

In simulation studies, we also benchmarked GMIL against a GLMM with a corresponding likelihood and two widely used nonlinear models: Random Forest and XGBoost. All models use predefined bag-level features as inputs, based on three different strategies: mean pooling, median pooling, and a combination of mean, squared mean, and cubed mean of instance features (Figure A1 (ii)).

## A3 Experimental setup

### A3.1 Simulations and Genomics dataset

**MIL model hyperparameter search.** Hyperparameters for all MIL models across the simulations and genomics application were optimized based on the simulation default scenario, which emulates the genomics dataset. Specifically, we used our simulation procedure with default parameters to generate 10 datasets, including training and validation sets. For each simulated dataset, we trained MIL models with different losses, learning rates and regularization parameters (Table A1) on the training set and evaluated their performance on the validation set. The hyperparameters for each model were then chosen based on the average Spearman correlation between predicted and true values, and are listed in Table A2. Across the losses that we considered, which included common regression losses (MSELoss, HuberLoss, SmoothL1Loss, L1Loss) as well as the negative log-likelihood of the Binomial distribution used in GMIL, the HuberLoss consistently yielded the best results for this use case.

Table A1: Hyperparameter sweep for Simulations and Genomics dataset

| Model       | Learning Rate            | Weight Decay                   | Dim. Encoder | Regularization          |
|-------------|--------------------------|--------------------------------|--------------|-------------------------|
| Bayes-MIL   | {5e-3, 1e-4, 5e-4, 1e-5} | {5e-4, 1e-4, 5e-5, 1e-5, 1e-6} | {30}         | log10space(1e-6, 1e-10) |
| DSMIL       | {5e-3, 2e-4, 5e-5}       | {5e-3, 5e-4, 1e-4}             | {30}         | -                       |
| ABMIL       | {5e-3, 5e-4, 5e-5}       | {5e-3, 5e-4, 1e-4, 1e-5, 0}    | {30}         | -                       |
| Gated ABMIL | {5e-3, 5e-4, 5e-5}       | {5e-3, 5e-4, 1e-4, 1e-5, 0}    | {30}         | -                       |

Table A2: Optimized Hyperparameters for Simulations and Genomics dataset

| Model       | Learning Rate | Weight Decay | Dim. Encoder | Regularization |
|-------------|---------------|--------------|--------------|----------------|
| Bayes-MIL   | 5e-4          | 1e-6         | 30           | 1e-8           |
| DSMIL       | 2e-4          | 5e-3         | 30           | -              |
| ABMIL       | 5e-4          | 1e-4         | 30           | -              |
| Gated ABMIL | 5e-4          | 1e-4         | 30           | -              |

**Traditional ML models hyperparameter search.** To tune the hyperparameters of the baseline models considered in our paper, we performed a randomized search of the hyperparameter space, using a 5-fold cross-validation within the training set and sampling 20 hyperparameter combinations. Specifically, each combination of hyperparameters was evaluated by the average cross-validated Spearman correlation metric, the combination that provided the best performance was chosen, and the final models were retrained on the entire training set before performing out-of-sample predictions on the test set. For full information on hyperparameters and their respective search spaces see Table A3 and Table A4.

Table A3: Random Forest Hyperparameter Search Space

| Hyperparameter                        | Search Space             |
|---------------------------------------|--------------------------|
| Number of Estimators (n_estimators)   | {50, 100, 150, 200, 500} |
| Max Features (max_features)           | {sqrt, log2, None}       |
| Max Depth (max_depth)                 | {10, 20, 30, 50}         |
| Min Samples Split (min_samples_split) | {2, 5, 10}               |
| Min Samples Leaf (min_samples_leaf)   | {1, 2, 4}                |

Table A4: XGBoost Hyperparameter Search Space

| Hyperparameter                        | Search Space                                 |
|---------------------------------------|----------------------------------------------|
| Max Depth (max_depth)                 | {3, 4, ..., 9}                               |
| Learning Rate (learning_rate)         | { $10^{-3}$ , ..., $10^{-2}$ , ..., $10^0$ } |
| Number of Estimators (n_estimators)   | (100, 1000)                                  |
| Subsample (subsample)                 | (0.5, 1)                                     |
| Col Sample By Tree (colsample_bytree) | (0.5, 1)                                     |
| Objective (objective)                 | binary:logistic                              |
| Evaluation Metric (eval_metric)       | logloss                                      |

### A3.2 Microscopy dataset

For the microscopy data, we ran three repeat experiments, each time holding out a different plate as a test set. For each repeat experiment, we trained MIL models with different hyperparameters on 90% of the training set (Table A5) and evaluated their predictive performance based on the F1 score on the remaining 10%. For each model, we considered hyperparameters that yielded the best performance on this validation set and retrained on the entire training set before computing predictions on the test set. We noticed that the same hyperparameters were selected for each model across the three repeat experiments (Table A6).

Table A5: Hyperparameter sweep for Microscopy Dataset

| Model          | Learning Rate      | Dim. Encoder   |
|----------------|--------------------|----------------|
| Bayes-MIL      | {1e-3, 5e-4, 1e-4} | {64, 100, 128} |
| DSMIL          | {1e-3, 5e-4, 1e-4} | {64, 100, 128} |
| ABMIL          | {1e-3, 5e-4, 1e-4} | {64, 100, 128} |
| Additive ABMIL | {1e-3, 5e-4, 1e-4} | {64, 100, 128} |
| Gated ABMIL    | {1e-3, 5e-4, 1e-4} | {64, 100, 128} |

Table A6: Optimized Hyperparameters for Microscopy Dataset

| Model          | Learning Rate | Weight Decay | Dim. Encoder |
|----------------|---------------|--------------|--------------|
| Bayes-MIL      | 1e-4          | 1e-5         | 64           |
| DSMIL          | 1e-4          | 1e-5         | 100          |
| ABMIL          | 5e-4          | 1e-5         | 100          |
| Additive ABMIL | 5e-4          | 1e-5         | 100          |
| Gated ABMIL    | 5e-4          | 1e-5         | 100          |

### A3.3 Histopathology dataset

We employed the version of Camelyon16 provided by (Li et al., 2021), which contained a predefined train-test split. We earmarked 10% of the training bags for hyperparameter optimization and swept MIL model hyperparameters using a grid-search approach (Table A7). For each model, we picked hyperparameters based on the validation loss. The final parameters are shown in Table A8.

Table A7: Hyperparameter sweep for Camelyon16 Dataset

| Model       | Learning Rate            | Weight Decay             | Dim. Encoder  | Regularization                       |
|-------------|--------------------------|--------------------------|---------------|--------------------------------------|
| Bayes-MIL   | {5e-4, 1e-4, 5e-5, 1e-5} | {1e-4, 1e-5, 1e-6, 1e-7} | {30, 60, 120} | $\log_{10}\text{space}(1e-6, 1e-10)$ |
| DSMIL       | {1e-4, 2e-4, 5e-5}       | {5e-3}                   | {30, 60, 120} | -                                    |
| ABMIL       | {1e-4, 5e-4, 5e-5}       | {1e-4}                   | {30, 60, 120} | -                                    |
| Gated ABMIL | {1e-4, 5e-4, 5e-5}       | {1e-4}                   | {30, 60, 120} | -                                    |

Table A8: Optimized Hyperparameters for Camelyon16 Dataset

| Model       | Learning Rate | Weight Decay | Dim. Encoder | Regularization |
|-------------|---------------|--------------|--------------|----------------|
| Bayes-MIL   | 5e-4          | 1e-5         | 30           | 1e-8           |
| DSMIL       | 1e-4          | 5e-3         | 60           | -              |
| ABMIL       | 5e-5          | 1e-4         | 60           | -              |
| Gated ABMIL | 5e-4          | 1e-4         | 30           | -              |

## A4 Data processing

### A4.1 Variant filtering procedure

To identify the 28 variants associated with the average transcriptional state, we adopted the following approach: We started from 16,718 variants associated with proximal gene expression in the primary analysis of this data. These variants are typically known as cis-expression Quantitative Trait Loci (cis-eQTLs). Then, we selected variants that could be predicted from average cell embedding using a GLMM (Spearman  $\rho > 0.15$ ). Next, to mitigate dependencies between genetic labels due to linkage disequilibrium (Slatkin, 2008), we undertook a clumping procedure (Purcell et al., 2007), which yielded the final set of 28 variants.

### A4.2 Single-cell Embeddings

Single-cell RNA-seq data consists of a cell-by-gene matrix of RNA counts per cell. For the OneK1K dataset, we have approximately 1.3 million cells and 32,000 genes (Yazar et al., 2022). However, due to technical bias and experimental dropout, many of these genes are uninformative. Therefore, it is common to subset to the most highly variable genes and perform analyses on embedding space. The single-cell Variational Inference (scVI) model (Lopez et al., 2018) is designed with the properties of this data in mind. We used hyperparameters commonly used for this type of dataset size and reported them in Table A9.

---

Table A9: Summary of scVI (Lopez et al., 2018) parameters

| Parameter                   | Value           |
|-----------------------------|-----------------|
| Layers                      | 2               |
| Batch Size                  | 256             |
| Epochs                      | 15              |
| Gene Likelihood             | ZINB            |
| Covariate                   | Sequencing Pool |
| Highly Variable Genes (HVG) | 5000            |

As described in the main, we performed the scVI integration on the sub-lymphoid cells (CD4, CD8, NK cells).

#### A4.3 Microscopy image feature extraction

We downloaded cell images from Caie et al. (2010), extracted single cell images using nuclear coordinates made available by Ljosa et al. (2013), and applied plate correction as described in Singh et al. (2014). We then collected the weights of a ResNet50 SimCLR model pre-trained by Perakis et al. (2021) to infer cell embeddings. The extracted embeddings have a dimensionality of 2048, which we reduce using PCA.

## A5 Additional Results

### A5.1 Simulations

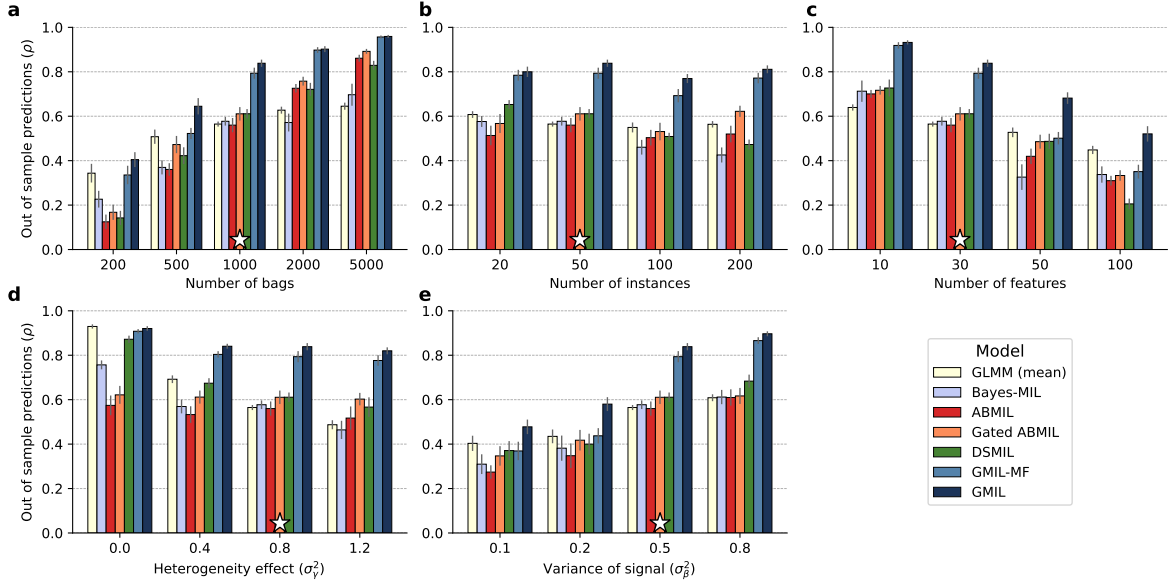

(i) Comparison with MIL models

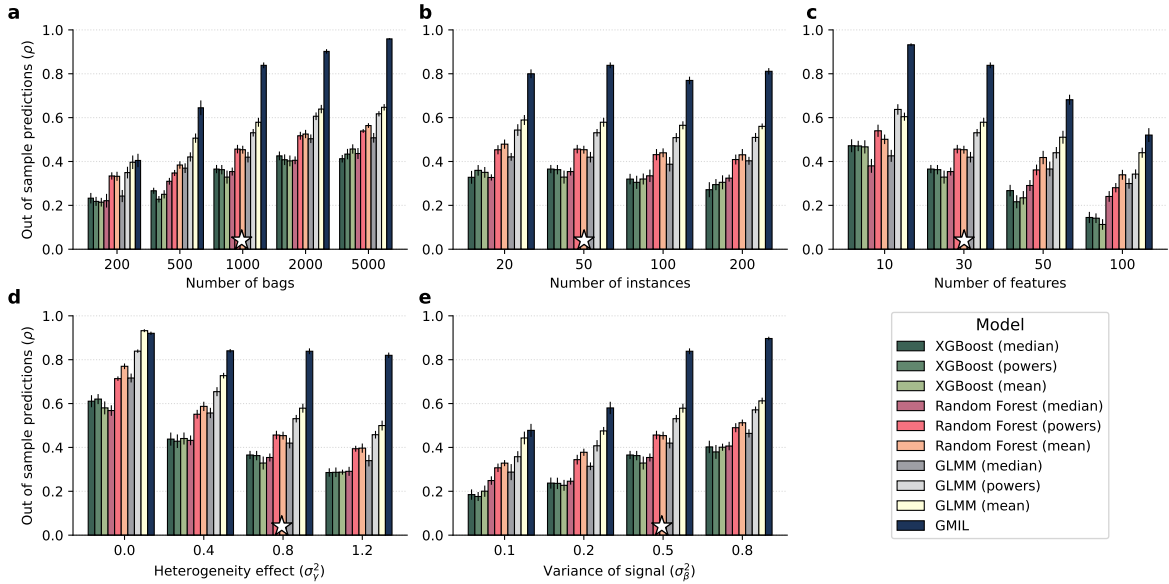

(ii) Comparison with vs GLMM, Random Forest, and XGBoost

Figure A1: Out-of-sample prediction performance (Spearman correlation,  $\rho$ ) in different simulation settings, varying one parameter at a time while keeping the others constant. Specifically, we varied the number of bags (a), the number of instances (b), the number of features (c), the heterogeneity effect (d) and the variance of signal (e).

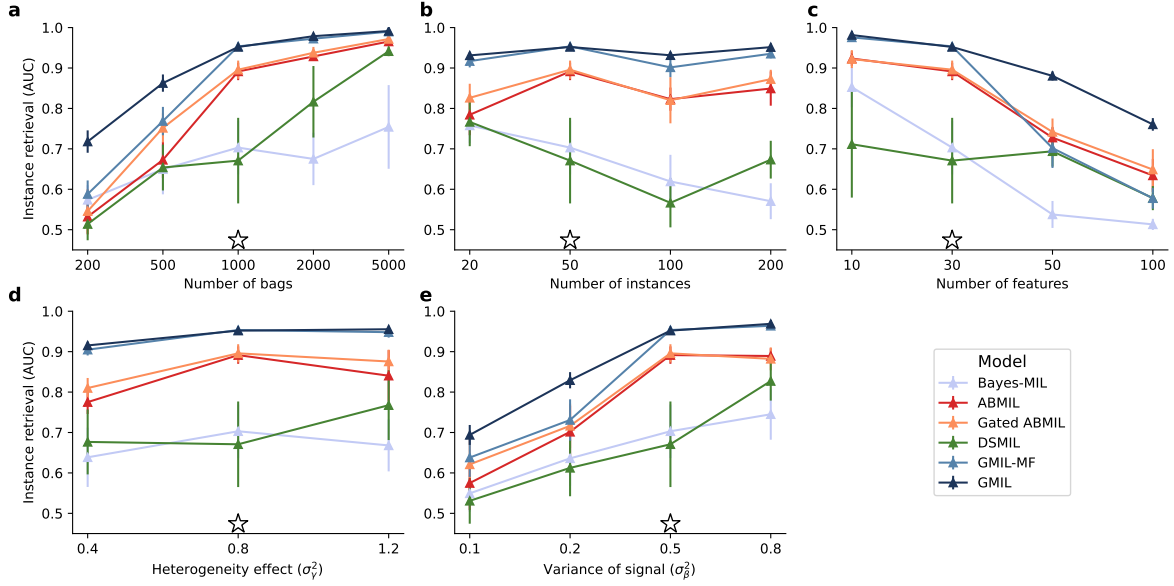

Figure A2: Instance retrieval ROC-AUC of GMIL for top 10% of instances in the same simulated scenarios. Error bars denote standard errors across 10 repeat experiments.

## A5.2 Single-cell Genomics dataset

Table A10: Comparison of prediction performance of GMIL and baseline MILs on the single-cell genomics data. The table reports the mean and standard deviation of Spearman correlation across 28 genes, and the p-values obtained from a paired t-test, assessing the statistical significance of the differences in performance between GMIL and each of the baseline MILs.

| Method      | Prediction performance (Spearman) | GMIL improvement (t-test p-value) |
|-------------|-----------------------------------|-----------------------------------|
| ABMIL       | $0.21 \pm 0.18$                   | $< 4 \cdot 10^{-7}$               |
| DSMIL       | $0.22 \pm 0.17$                   | $< 2 \cdot 10^{-7}$               |
| Bayes-MIL   | $0.23 \pm 0.14$                   | $< 2 \cdot 10^{-4}$               |
| Gated ABMIL | $0.24 \pm 0.18$                   | $< 5 \cdot 10^{-6}$               |
| GMIL        | <b><math>0.29 \pm 0.17</math></b> | -                                 |

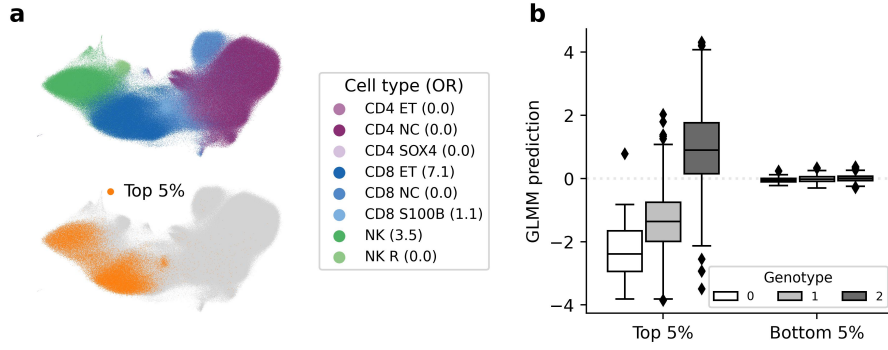

(i) **rs12151621** (Chromosome 2, near GNLY (Tewary et al., 2010)). Differential gene analysis brought up processes related to defence response (GO:0031349) and regulation of the MAPK cascade (GO:0043408, Plotnikov et al. (2011)).

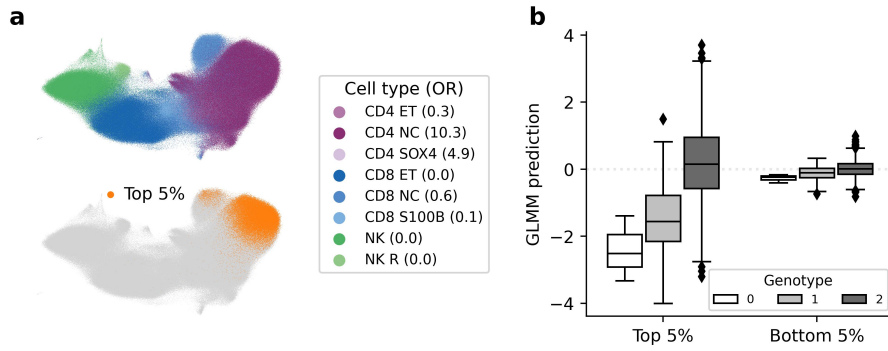

(ii) **rs9928554** (Chromosome 16, near IL32), associated with Vitamin E measurements (openTargets, Ochoa et al. (2023)). Differential gene analysis brought up processes related to protein transport to the membrane (GO:0072657) and cell regulatory processes (GO:0050728, GO:0043408, GO:0031349).

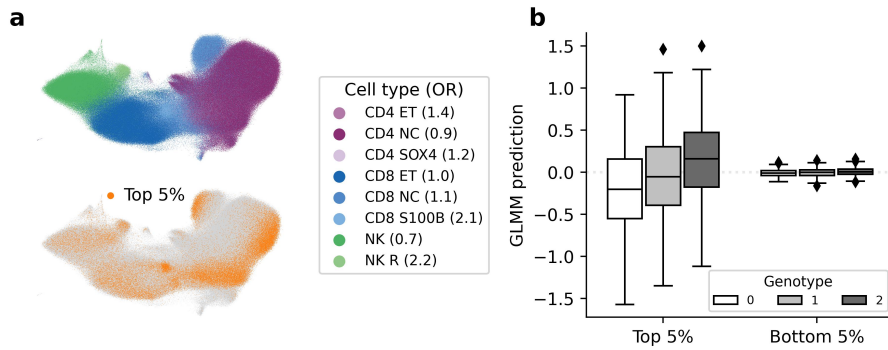

(iii) **rs7503161** (Chromosome 17, near EIF5A) associated with increased hemoglobin concentration and height (openTargets, Ochoa et al. (2023)). EIF5A is involved in the positive regulation of the apoptosis (programmed cell death) signaling pathway. Differential gene analysis yielded processes directly (GO:0042981, GO:0043069, GO:0043066) and indirectly (GO:0071345, GO:1902531) related to cell death.

Figure A3: Three examples of genetic variants for which GMIL improved predictions. (a) UMAP of cell transcriptional embeddings showing cell types (top panel) and top 5% relevant cells according to GMIL's weights (bottom panel). The odds ratio (OR) quantifies the enrichment of top-weighted cells within each cell type. (b) Box plots showing GLMM genetic predictions vs observed values, where the GLMM was fit either using the top 5% of the instances (left) or the bottom 5% (right) as ranked by GMIL. Panels (i) and (ii) show variants where GMIL's importance weights align with known cell types. Conversely, panel (iii) finds a cell state not captured by any individual cell type.



### A5.3 Microscopy dataset

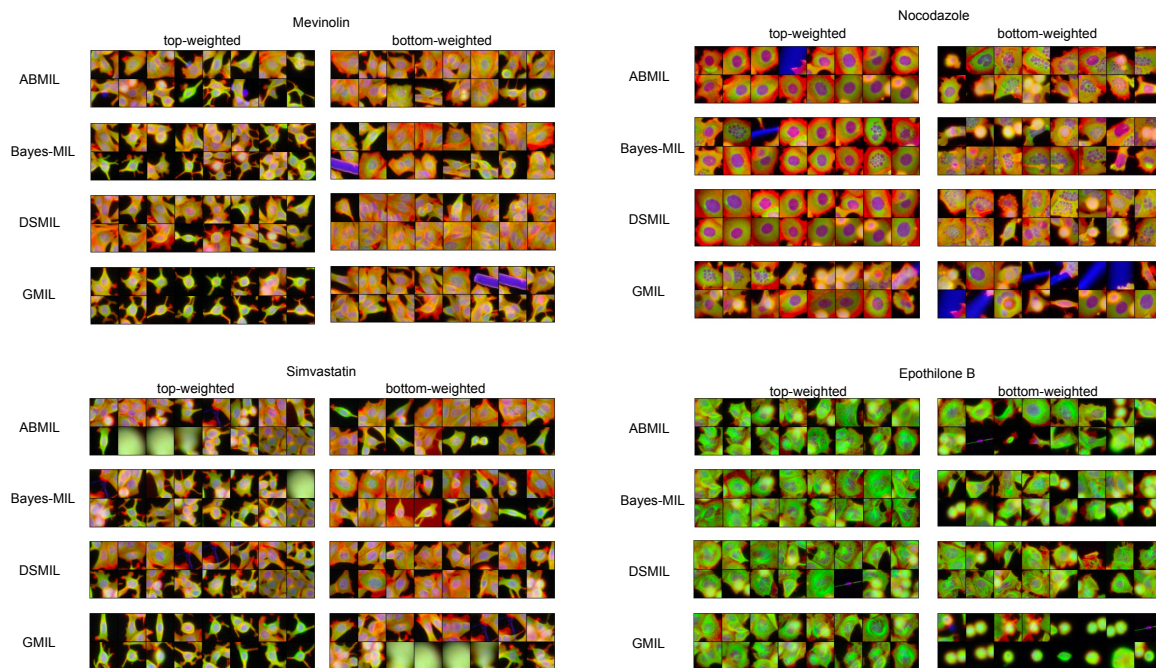

Figure A4: Top and bottom 16 weighted cells for the Nocodazole, Simvastatin, Epothilone B and Mevinolin for different MIL methods. While GMIL down-weights images with technical artefacts and yields consistent phenotypes in the top classes, the competing MIL models tend to miss or up-weight noisy images and produce inconsistent phenotypes for the most important perturbed images.

Table A11: F1 score comparison between GMIL and competing MIL models on individual MoA labels. We observe that GMIL improves on the MIL baselines on most considered classes.

| MoA Category              | Method         | F1                                  |
|---------------------------|----------------|-------------------------------------|
| Actin Disruptors          | ABMIL          | 0.841 $\pm$ 0.014                   |
|                           | Additive ABMIL | 0.235 $\pm$ 0.121                   |
|                           | Bayes-MIL      | 0.733 $\pm$ 0.035                   |
|                           | DSMIL          | 0.920 $\pm$ 0.025                   |
|                           | Gated ABMIL    | 0.730 $\pm$ 0.040                   |
|                           | <b>GMIL</b>    | <b>0.992 <math>\pm</math> 0.004</b> |
| Aurora Kinase Inhibitors  | ABMIL          | 0.910 $\pm$ 0.013                   |
|                           | Additive ABMIL | 0.600 $\pm$ 0.155                   |
|                           | Bayes-MIL      | 0.862 $\pm$ 0.011                   |
|                           | DSMIL          | 0.970 $\pm$ 0.008                   |
|                           | Gated ABMIL    | 0.783 $\pm$ 0.034                   |
|                           | <b>GMIL</b>    | <b>1.000 <math>\pm</math> 0.000</b> |
| Cholesterol-Lowering      | ABMIL          | 0.550 $\pm$ 0.026                   |
|                           | Additive ABMIL | 0.562 $\pm$ 0.023                   |
|                           | Bayes-MIL      | 0.293 $\pm$ 0.059                   |
|                           | DSMIL          | 0.885 $\pm$ 0.008                   |
|                           | Gated ABMIL    | 0.415 $\pm$ 0.011                   |
|                           | <b>GMIL</b>    | <b>0.914 <math>\pm</math> 0.001</b> |
| DNA Damage                | ABMIL          | 0.711 $\pm$ 0.009                   |
|                           | Additive ABMIL | 0.316 $\pm$ 0.101                   |
|                           | Bayes-MIL      | 0.715 $\pm$ 0.027                   |
|                           | DSMIL          | 0.882 $\pm$ 0.016                   |
|                           | Gated ABMIL    | 0.558 $\pm$ 0.071                   |
|                           | <b>GMIL</b>    | <b>0.922 <math>\pm</math> 0.019</b> |
| DNA Replication           | ABMIL          | 0.677 $\pm$ 0.013                   |
|                           | Additive ABMIL | 0.595 $\pm$ 0.015                   |
|                           | Bayes-MIL      | 0.712 $\pm$ 0.012                   |
|                           | DSMIL          | 0.838 $\pm$ 0.030                   |
|                           | Gated ABMIL    | 0.542 $\pm$ 0.039                   |
|                           | <b>GMIL</b>    | <b>0.928 <math>\pm</math> 0.010</b> |
| Eg5 Inhibitors            | ABMIL          | 0.868 $\pm$ 0.004                   |
|                           | Additive ABMIL | 0.457 $\pm$ 0.118                   |
|                           | Bayes-MIL      | 0.825 $\pm$ 0.006                   |
|                           | DSMIL          | 0.947 $\pm$ 0.006                   |
|                           | Gated ABMIL    | 0.859 $\pm$ 0.014                   |
|                           | <b>GMIL</b>    | <b>0.993 <math>\pm</math> 0.004</b> |
| Epithelial                | ABMIL          | 0.759 $\pm$ 0.023                   |
|                           | Additive ABMIL | 0.000 $\pm$ 0.000                   |
|                           | Bayes-MIL      | 0.631 $\pm$ 0.026                   |
|                           | DSMIL          | 0.865 $\pm$ 0.012                   |
|                           | Gated ABMIL    | 0.722 $\pm$ 0.026                   |
|                           | <b>GMIL</b>    | <b>0.929 <math>\pm</math> 0.008</b> |
| Kinase Inhibitors         | ABMIL          | 0.673 $\pm$ 0.040                   |
|                           | Additive ABMIL | 0.000 $\pm$ 0.000                   |
|                           | Bayes-MIL      | 0.503 $\pm$ 0.048                   |
|                           | <b>DSMIL</b>   | <b>0.956 <math>\pm</math> 0.010</b> |
|                           | Gated ABMIL    | 0.658 $\pm$ 0.032                   |
|                           | GMIL           | 0.927 $\pm$ 0.019                   |
| Microtubule Destabilizers | ABMIL          | 0.769 $\pm$ 0.019                   |
|                           | Additive ABMIL | 0.621 $\pm$ 0.024                   |
|                           | Bayes-MIL      | 0.701 $\pm$ 0.012                   |
|                           | DSMIL          | 0.932 $\pm$ 0.002                   |
|                           | Gated ABMIL    | 0.816 $\pm$ 0.009                   |
|                           | <b>GMIL</b>    | <b>0.968 <math>\pm</math> 0.006</b> |
| Microtubule Stabilizers   | ABMIL          | 0.932 $\pm$ 0.014                   |
|                           | Additive ABMIL | 0.283 $\pm$ 0.146                   |
|                           | Bayes-MIL      | 0.858 $\pm$ 0.013                   |
|                           | DSMIL          | 0.964 $\pm$ 0.006                   |
|                           | Gated ABMIL    | 0.822 $\pm$ 0.020                   |
|                           | <b>GMIL</b>    | <b>1.000 <math>\pm</math> 0.000</b> |
| Protein Degradation       | ABMIL          | 0.312 $\pm$ 0.020                   |
|                           | Additive ABMIL | 0.292 $\pm$ 0.038                   |
|                           | Bayes-MIL      | 0.275 $\pm$ 0.027                   |
|                           | DSMIL          | 0.688 $\pm$ 0.054                   |
|                           | Gated ABMIL    | 0.321 $\pm$ 0.037                   |
|                           | <b>GMIL</b>    | <b>0.773 <math>\pm</math> 0.026</b> |
| Protein Synthesis         | ABMIL          | 0.757 $\pm$ 0.023                   |
|                           | Additive ABMIL | 0.076 $\pm$ 0.039                   |
|                           | Bayes-MIL      | 0.447 $\pm$ 0.041                   |
|                           | DSMIL          | 0.879 $\pm$ 0.008                   |
|                           | Gated ABMIL    | 0.625 $\pm$ 0.016                   |
|                           | <b>GMIL</b>    | <b>0.960 <math>\pm</math> 0.006</b> |

Table A12: Comparison of GMIL and MIL baseline models with varying numbers of embedding principal components based on balanced accuracy, F1-macro, and F1-micro, including confidence intervals. Consistent with previous scenarios, GMIL outperforms other approaches on all evaluated feature dimensions.

| Method         | Number of Features | Balanced Accuracy                   | F1-macro                            | F1-micro                            |
|----------------|--------------------|-------------------------------------|-------------------------------------|-------------------------------------|
| ABMIL          | 64                 | $0.581 \pm 0.036$                   | $0.577 \pm 0.041$                   | $0.607 \pm 0.047$                   |
|                | 256                | $0.726 \pm 0.018$                   | $0.730 \pm 0.016$                   | $0.764 \pm 0.015$                   |
|                | 512                | $0.714 \pm 0.010$                   | $0.709 \pm 0.013$                   | $0.746 \pm 0.009$                   |
| Additive ABMIL | 64                 | $0.298 \pm 0.022$                   | $0.203 \pm 0.020$                   | $0.340 \pm 0.028$                   |
|                | 256                | $0.410 \pm 0.003$                   | $0.336 \pm 0.002$                   | $0.470 \pm 0.019$                   |
|                | 512                | $0.475 \pm 0.045$                   | $0.379 \pm 0.051$                   | $0.501 \pm 0.051$                   |
| Bayes-MIL      | 64                 | $0.727 \pm 0.042$                   | $0.733 \pm 0.044$                   | $0.758 \pm 0.031$                   |
|                | 256                | $0.623 \pm 0.018$                   | $0.628 \pm 0.024$                   | $0.699 \pm 0.014$                   |
|                | 512                | $0.641 \pm 0.005$                   | $0.642 \pm 0.010$                   | $0.693 \pm 0.011$                   |
| DSMIL          | 64                 | $0.849 \pm 0.028$                   | $0.850 \pm 0.026$                   | $0.859 \pm 0.022$                   |
|                | 256                | $0.892 \pm 0.025$                   | $0.894 \pm 0.023$                   | $0.902 \pm 0.019$                   |
|                | 512                | $0.890 \pm 0.018$                   | $0.895 \pm 0.018$                   | $0.908 \pm 0.014$                   |
| Gated ABMIL    | 64                 | $0.528 \pm 0.016$                   | $0.508 \pm 0.016$                   | $0.582 \pm 0.032$                   |
|                | 256                | $0.669 \pm 0.031$                   | $0.654 \pm 0.032$                   | $0.701 \pm 0.031$                   |
|                | 512                | $0.674 \pm 0.029$                   | $0.676 \pm 0.027$                   | $0.707 \pm 0.027$                   |
| GMIL           | <b>64</b>          | <b><math>0.912 \pm 0.019</math></b> | <b><math>0.915 \pm 0.018</math></b> | <b><math>0.924 \pm 0.017</math></b> |
|                | <b>256</b>         | <b><math>0.939 \pm 0.017</math></b> | <b><math>0.942 \pm 0.015</math></b> | <b><math>0.950 \pm 0.013</math></b> |
|                | <b>512</b>         | <b><math>0.939 \pm 0.019</math></b> | <b><math>0.944 \pm 0.016</math></b> | <b><math>0.951 \pm 0.014</math></b> |

## References

- Peter D. Caie, Rebecca E. Walls, Alexandra Ingleston-Orme, et al. High-content phenotypic profiling of drug response signatures across distinct cancer cells. Molecular Cancer Therapeutics, 9(6), June 2010.
- Yufei Cui, Ziquan Liu, Xiangyu Liu, Xue Liu, Cong Wang, Tei-Wei Kuo, Chun Jason Xue, and Antoni B. Chan. Bayes-MIL: A new probabilistic perspective on attention-based multiple instance learning for whole slide images. In The Eleventh International Conference on Learning Representations, 2023.
- Maximilian Ilse, Jakub Tomczak, and Max Welling. Attention-based deep multiple instance learning. In International conference on machine learning. PMLR, 2018.
- Syed Ashar Javed, Dinkar Juyal, Harshith Padigela, Amaro Taylor-Weiner, Limin Yu, and Aaditya Prakash. Additive mil: Intrinsically interpretable multiple instance learning for pathology. In S. Koyejo, S. Mohamed, A. Agarwal, D. Belgrave, K. Cho, and A. Oh, editors, Advances in Neural Information Processing Systems, volume 35. Curran Associates, Inc., 2022.
- Bin Li, Yin Li, and Kevin W. Eliceiri. Dual-stream multiple instance learning network for whole slide image classification with self-supervised contrastive learning. In Proceedings of the IEEE/CVF Conference on Computer Vision and Pattern Recognition (CVPR), June 2021.
- Vebjorn Ljosa, Peter D Caie, Rob Ter Horst, Katherine L Sokolnicki, Emma L Jenkins, Sandeep Daya, Mark E Roberts, Thouis R Jones, Shantanu Singh, Auguste Genovesio, et al. Comparison of methods for image-based profiling of cellular morphological responses to small-molecule treatment. Journal of biomolecular screening, 18(10), 2013.
- Romain Lopez, Jeffrey Regier, Michael B Cole, et al. Deep generative modeling for single-cell transcriptomics. Nature Methods, 15(12), 2018.
- David Ochoa, Andrew Hercules, Miguel Carmona, Daniel Suveges, Jarrod Baker, Cinzia Malangone, Irene Lopez, Alfredo Miranda, Carlos Cruz-Castillo, Luca Fumis, et al. The next-generation open targets platform: reimaged, redesigned, rebuilt. Nucleic acids research, 51(D1):D1353–D1359, 2023.
- Alexis Perakis, Ali Gorji, Samriddhi Jain, et al. Contrastive learning of single-cell phenotypic representations for treatment classification. In Machine Learning in Medical Imaging. Springer International Publishing, 2021.
- Alexander Plotnikov, Eldar Zehorai, Shiri Procaccia, and Rony Seger. The mapk cascades: Signaling components, nuclear roles and mechanisms of nuclear translocation. Biochimica et Biophysica Acta (BBA) - Molecular Cell Research, 1813(9), 2011. Regulation of Signaling and Cellular Fate through Modulation of Nuclear Protein Import.
- Shaun Purcell, Benjamin Neale, Kathe Todd-Brown, Lori Thomas, Manuel AR Ferreira, David Bender, Julian Maller, Pamela Sklar, Paul IW De Bakker, Mark J Daly, et al. Plink: a tool set for whole-genome association and population-based linkage analyses. The American journal of human genetics, 81(3), 2007.
- S. Singh, M.-A. Bray, T.R. Jones, and A.E. Carpenter. Pipeline for illumination correction of images for high-throughput microscopy. Journal of Microscopy, 256(3), September 2014.
- Montgomery Slatkin. Linkage disequilibrium—understanding the evolutionary past and mapping the medical future. Nature Reviews Genetics, 9(6), 2008.
- Poonam Tewary, De Yang, Gonzalo de la Rosa, Yana Li, Michael W. Finn, Alan M. Krensky, Carol Clayberger, and Joost J. Oppenheim. Granulysin activates antigen-presenting cells through TLR4 and acts as an immune alarmin. Blood, 116(18), 11 2010.
- Seyhan Yazar, Jose Alquicira-Hernandez, Kristof Wing, et al. Single-cell eqtl mapping identifies cell type-specific genetic control of autoimmune disease. Science, 376(6589), 2022.

---

## Checklist

1. For all models and algorithms presented, check if you include:
  - (a) A clear description of the mathematical setting, assumptions, algorithm, and/or model. [Yes/No/Not Applicable]
  - (b) An analysis of the properties and complexity (time, space, sample size) of any algorithm. [Yes/No/Not Applicable]
  - (c) (Optional) Anonymized source code, with specification of all dependencies, including external libraries. [Yes/No/Not Applicable]
2. For any theoretical claim, check if you include:
  - (a) Statements of the full set of assumptions of all theoretical results. [Yes/No/Not Applicable]
  - (b) Complete proofs of all theoretical results. [Yes/No/Not Applicable]
  - (c) Clear explanations of any assumptions. [Yes/No/Not Applicable]
3. For all figures and tables that present empirical results, check if you include:
  - (a) The code, data, and instructions needed to reproduce the main experimental results (either in the supplemental material or as a URL). [Yes/No/Not Applicable]
  - (b) All the training details (e.g., data splits, hyperparameters, how they were chosen). [Yes/No/Not Applicable]
  - (c) A clear definition of the specific measure or statistics and error bars (e.g., with respect to the random seed after running experiments multiple times). [Yes/No/Not Applicable]
  - (d) A description of the computing infrastructure used. (e.g., type of GPUs, internal cluster, or cloud provider). [Yes/No/Not Applicable]
4. If you are using existing assets (e.g., code, data, models) or curating/releasing new assets, check if you include:
  - (a) Citations of the creator If your work uses existing assets. [Yes/No/Not Applicable]
  - (b) The license information of the assets, if applicable. [Yes/No/Not Applicable]
  - (c) New assets either in the supplemental material or as a URL, if applicable. [Yes/No/Not Applicable]
  - (d) Information about consent from data providers/curators. [Yes/No/Not Applicable]
  - (e) Discussion of sensible content if applicable, e.g., personally identifiable information or offensive content. [Yes/No/Not Applicable]
5. If you used crowdsourcing or conducted research with human subjects, check if you include:
  - (a) The full text of instructions given to participants and screenshots. [Yes/No/Not Applicable]
  - (b) Descriptions of potential participant risks, with links to Institutional Review Board (IRB) approvals if applicable. [Yes/No/Not Applicable]
  - (c) The estimated hourly wage paid to participants and the total amount spent on participant compensation. [Yes/No/Not Applicable]
